# Supplementary material for: Out-of-plane spin-to-charge conversion at low temperatures in graphene/MoTe$_2$ heterostructures
Source: arXiv:2309.00984 ancillary file (2023-09-02)
Supplement: Supplementary file 1 [file Ontoso_MoTe2_low_temperature_out_of_plane_Supporting.pdf]

# Supplementary material for

# *Out-of-plane spin-to-charge conversion at low temperatures in graphene/$MoTe_2$ heterostructures*

Nerea Ontoso,[1] C.K. Safeer,[1,2] Josep Ingla-Aynés,[1,3] Franz Herling,[1,4]
Luis E. Hueso,[1,5] M. Reyes Calvo,[6,7] and Fèlix Casanova[1,5]

[1]*CIC nanoGUNE BRTA, 20018 Donostia-San Sebastian, Basque Country, Spain*

[2]*Present address: Department of Physics, Clarendon Laboratory, University of Oxford, Oxford, United Kingdom*

[3]*Present address: Kavli Institute of Nanoscience, Delft University of Technology, 2628 CJ Delft, The Netherlands*

[4]*Present address: Catalan Institute of Nanoscience and Nanotechnology (ICN2), 08193 Barcelona, Spain*

[5]*IKERBASQUE, Basque Foundation for Science, 48009 Bilbao, Basque Country, Spain*

[6]*Departamento de Física Aplicada, Universidad de Alicante, 03690 Alicante, Spain*

[7]*Instituto Universitario de Materiales de Alicante (IUMA), Universidad de Alicante, 03690 Alicante, Spain*

(*f.casanova@nanogune.eu)

(*reyes.calvo@ua.es)

## S1. Spin Hall conductivity tensor for 1T' phase $MoTe_2$

In the Spin Hall effect, upon applying an electric field, a spin current is generated following:

$$j_i^{\alpha} = \sigma_{ij}^{\alpha} E_j, \tag{1}$$

where $j_i^{\alpha}$ is the spin current along the $i$-direction with spin polarization along $\alpha$-direction generated when an external electric field ($E_j$) along the $j$-direction is applied and $\sigma_{ij}^{\alpha}$ denotes the spin Hall conductivity tensor.

For the 1T' phase, the spin Hall conductivity tensor $\sigma_{ij}^{\alpha}$ is given by:

$$\sigma_{ij}^{x} = \begin{pmatrix} 0 & \sigma_{xy}^{x} & 0 \\ \sigma_{yx}^{x} & 0 & \sigma_{yz}^{x} \\ 0 & \sigma_{zy}^{x} & 0 \end{pmatrix} \quad \sigma_{ij}^{y} = \begin{pmatrix} \sigma_{xx}^{y} & 0 & \sigma_{xz}^{y} \\ 0 & \sigma_{yy}^{y} & 0 \\ \sigma_{zx}^{y} & 0 & \sigma_{zz}^{y} \end{pmatrix}$$

$$\sigma_{ij}^{z} = \begin{pmatrix} 0 & \sigma_{xy}^{z} & 0 \\ \sigma_{yx}^{z} & 0 & \sigma_{yz}^{z} \\ 0 & \sigma_{zy}^{z} & 0 \end{pmatrix}$$

where the 13 granted elements are independent.

## S2. Comparison to higher temperature data

Figure S1 shows a comparative of the low temperature data to a similar analysis of the high temperature data reported in Ref. [**?** ]

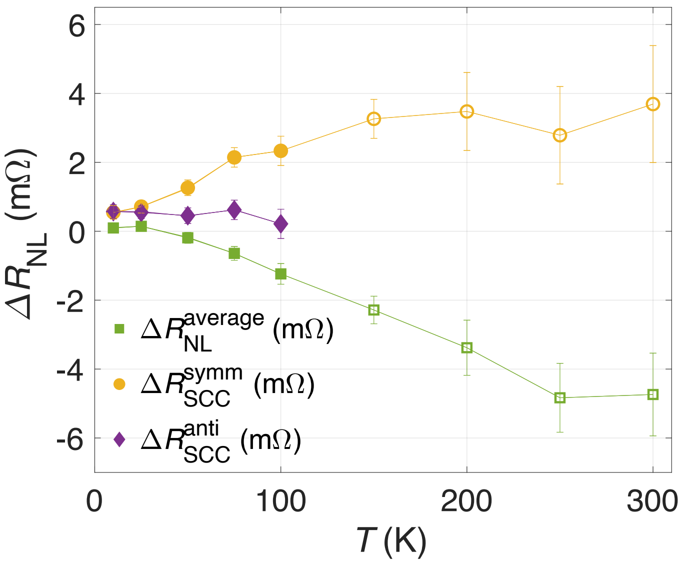


Fig. S1. Temperature dependence of the amplitude of the different contributions to $R_{\mathrm{NL}}$. The low temperature data (10 K - 100 K), represented by filled markers, are shown in Fig. 4. The higher temperature results (150 K - 300 K), represented by empty markers, are extracted from Ref. [**?** ], applying the analysis proposed in this work. The signal $R_{NL}^{average}$ is associated to the SCC of $s^x$, $R_{SCC}^{anti}$ is the contribution arising from $s^z$, and $R_{SCC}^{symm}$ from $s^y$. At temperatures above 100 K, the conversion of out-of-plane spins $s^z$ is below noise level. Error bars are calculated from the standard deviation of the signal noise.

## S3. Atomic force microscopy of graphene/$MoTe_2$ Device 1

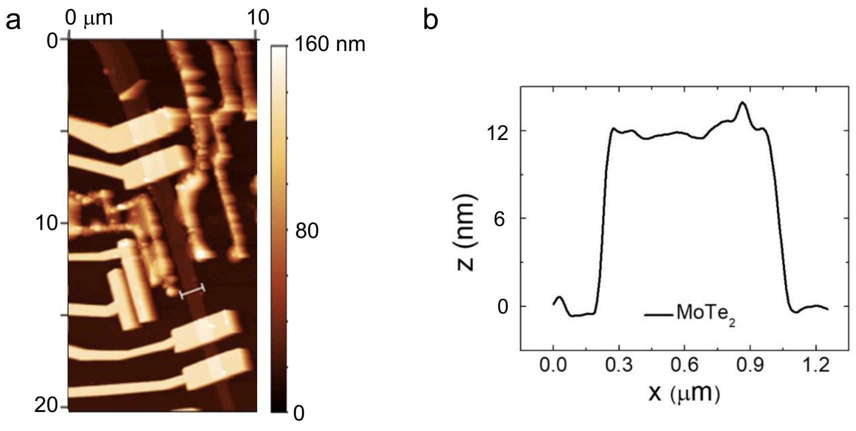


Fig. S2. a) Atomic force microscopy topography of the Device 1. b) Height profile for the line marked in white in panel (a)

## S4. Spin-to-charge conversion in Device 2

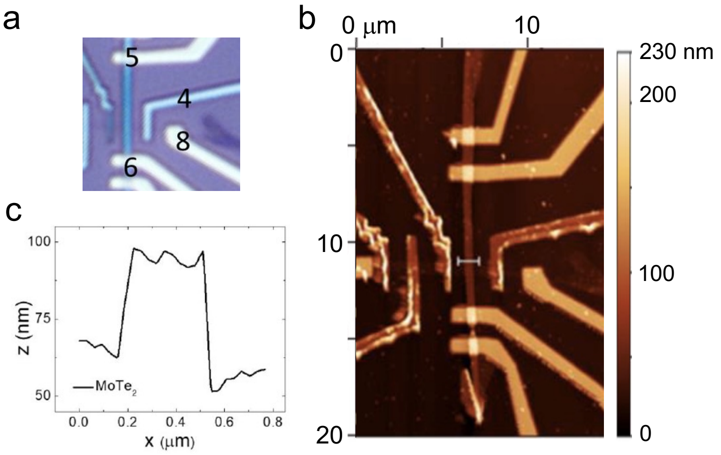


Fig. S3. a) Optical microscope image of Device 2. b) Atomic force microscopy topography of Device 2. c) Height profile for the line marked in white in panel (b)

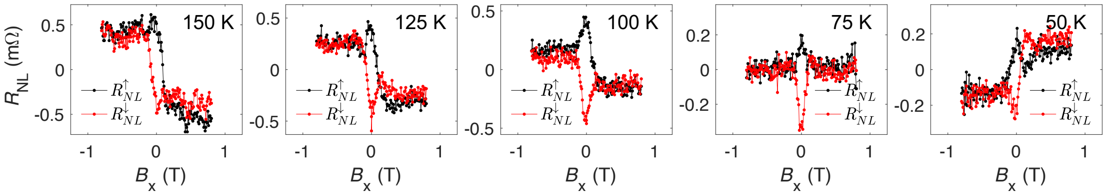


Fig. S4. Non-local resistance $R_{NL}$ measured while sweeping the magnetic field in the in-plane FM hard axis *x*-direction (see main text Figure 1b) for Device 2. Curves are presented for initial magnetization of the Co electrode saturated along positive (black) and negative (red) *y*-direction. Measurements were performed at the temperature indicated in each panel.

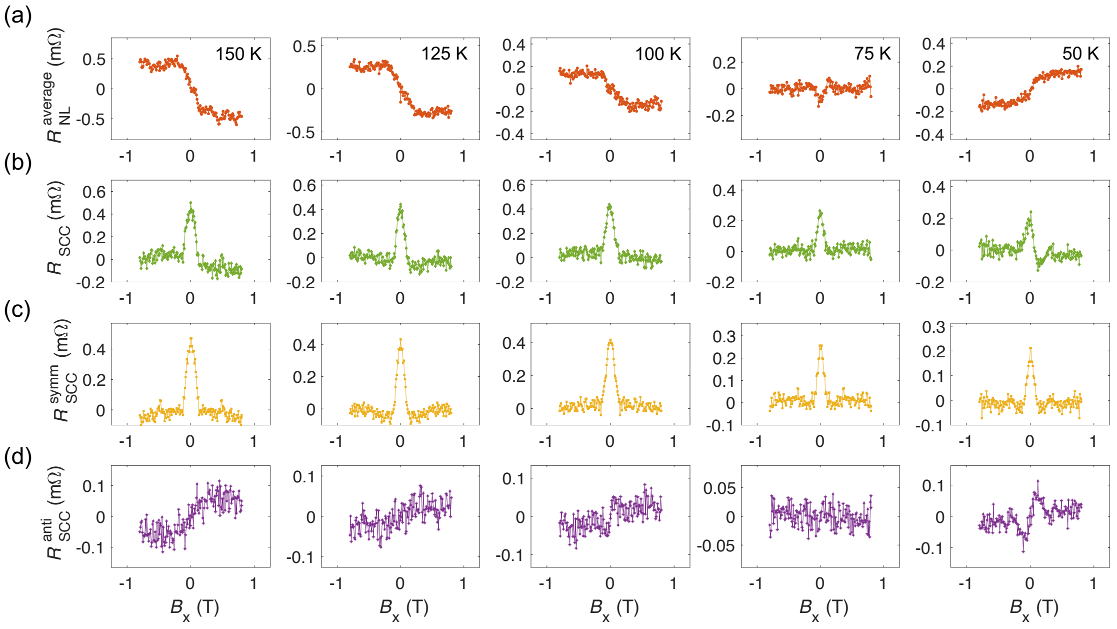


Fig. S5. (a) Average non-local resistance, defined as $R_{NL}^{average} = (R_{NL}^{\uparrow} + R_{NL}^{\downarrow})/2$ calculated from $R_{NL}$ data presented in Fig. S4 (b) Spin-to-charge conversion resistance defined as $R_{SCC} = (R_{NL}^{\uparrow} - R_{NL}^{\downarrow})/2$. (c) Symmetric component of the $R_{SCC}$ signal obtained from data in panel e. (d) Anti-symmetric component of the $R_{SCC}$ signal obtained from data in panel e. All signals are measured at the indicated temperatures.

## S5. Supplementary references

[1] C. K. Safeer, N. Ontoso, J. Ingla-Aynès, F. Herling, V. T. Pham, A. Kurzmann, K. Ensslin, A. Chuvilin, I. Robredo, M. G. Vergniory, F. de Juan, L. E. Hueso, M. R. Calvo, and F. Casanova, Nano Letters 19, 8758 (2019).
